# Supplementary material for: Optimal design of nanomagnets for on-chip field gradients
Source: arXiv:2212.13156 ancillary file (2022-12-26)
Supplement: Supplementary file 1 [file SpinQ_Nanomagnets_supp_subm1.pdf]

# Supplemental Material

—

# Optimal design of nanomagnets for on-chip field gradients

W. Legrand,[1,*] S. Lopes,[1,2,*] Q. Schaeverbeke,[1] F. Montaigne,[2] and M. M. Desjardins[1]

[1] *C12 Quantum Electronics, Paris, France*

[2] *Université de Lorraine, Institut Jean Lamour, UMR CNRS 7198, Nancy 54011, France*

## CONTENTS

S1. Definition of coordinates system for the ideal distribution calculations 2

S2. Additional representations for a transverse gradient ideal distribution 3

S3. Role of magnet thickness and interdot spacing 4

S4. Micromagnetic simulations and states at equilibrium 5

S5. Extraction of the stray fields and calculation of the coupling constants 7

References 7

* These two authors contributed equally

## S1. DEFINITION OF COORDINATES SYSTEM FOR THE IDEAL DISTRIBUTION CALCULATIONS

In Supp. Fig. S1, the definitions for the coordinates system and the different relevant angles are presented schematically, in the case of a $B_u$ or a $B_v$ field or gradient.

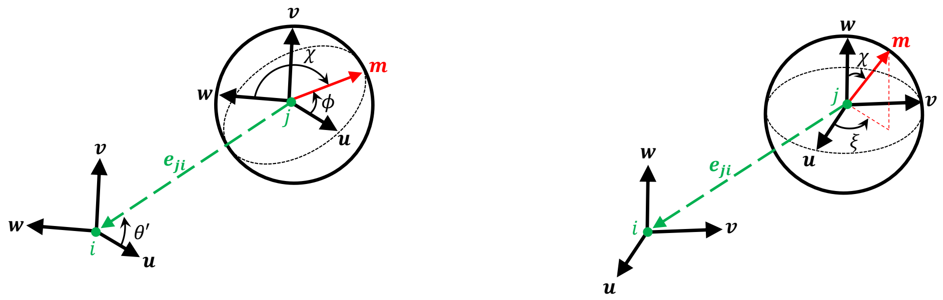


FIG. S1. Definition of coordinates system, considered plane and angles. (a) Case of a $B_u$ field or longitudinal gradient. All relevant angles $\theta'$ and $\phi$ are obtained in the plane defined by $\mathbf{u}$ and $\mathbf{e}_{ij}$. (b) General case, used for a transverse gradient, where no such plane reduction is possible. .

## S2. ADDITIONAL REPRESENTATIONS FOR A TRANSVERSE GRADIENT IDEAL DISTRIBUTION

We present below additional representations for the lower symmetry case of a transverse gradient generation with $\mathrm{d}Q = \mathrm{d}\partial\mathbf{B}_{ji} \cdot \hat{\mathbf{v}}/\partial u$. The plots display different planes offset from zero. The other cuts without offset, $(u, w)$ and $(v, w)$ planes, are not shown as they are either uniformly 0, or +1 and -1 either side of zero for $m_{\mathrm{u}}$, $m_{\mathrm{v}}$ and $m_{\mathrm{w}}$.

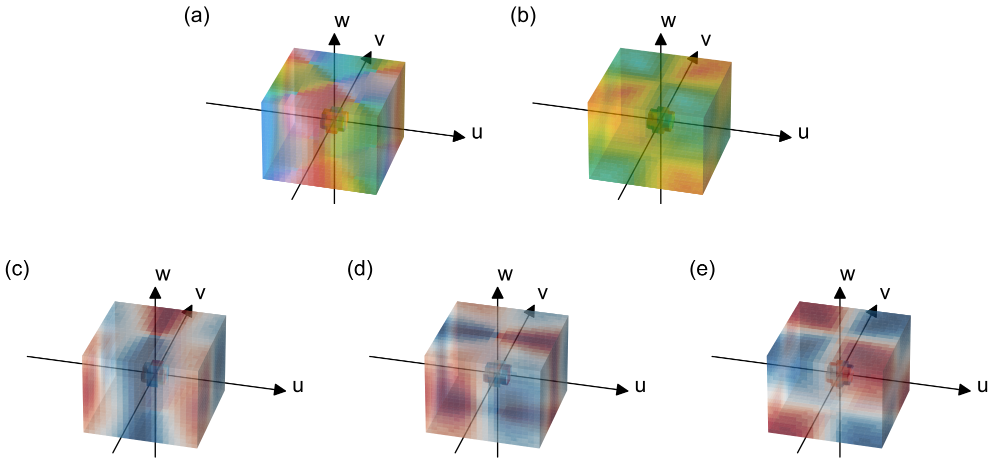


FIG. S2. Full views of the ideal magnetic distributions for optimising $\partial B_v/\partial u(0)$. (a) shows the in-plane angle $\xi$, (b) shows the out-of-plane angle $\chi$, (c) shows $m_{\mathrm{u}}$, (d) shows $m_{\mathrm{v}}$, (e) shows $m_{\mathrm{w}}$. Axes arrows for $u$, $v$ and $w$ have the same relative length.

## S3. ROLE OF MAGNET THICKNESS AND INTERDOT SPACING

The thickness of the magnetic layer and the spacing between the dots are fixed parameters in what is presented in the main text. In order to discuss the influence of these parameters on the $\sigma_{\mathrm{as}}$ term, we again consider a pair of nanowire quantum dots with linear confinement along the $x$ axis, located 100 nm above a magnetic layer of finite thickness. Similar to the example of the main text, we optimize $Q = \int B_z(x)\,|\psi_{\mathrm{L}}(x)|^2\,\mathrm{d}x - \int B_z(x)\,|\psi_{\mathrm{R}}(x)|^2\,\mathrm{d}x$ to take into account the spatial extension of the dots.

We compute the coupling constant $\alpha_{\mathrm{as}}$ for different interdot spacing values and magnetic layer thicknesses. The results are presented in Supp. Fig. S3(a) and Supp. Fig. S3(b), respectively.

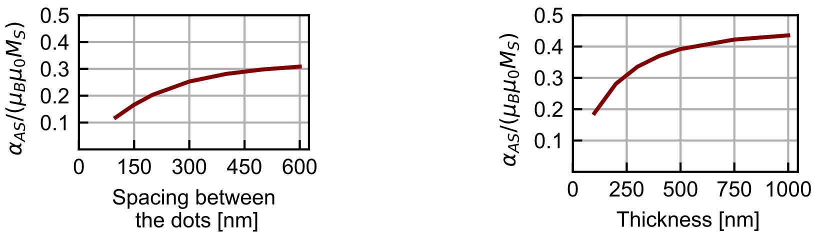


FIG. S3. Role of additional parameters in achieving a large field difference between the dots. (a) $\alpha_{\mathrm{as}}$ as a function of interdot spacing, fixed thickness of the magnetic layer of 200 nm. (b) $\alpha_{\mathrm{as}}$ as a function of thickness of the magnetic layer, fixed interdot spacing at 400 nm.

In Supp. Fig. S3(a), the interdot spacing is varied for a fixed thickness of the magnetic layer of 200 nm. Starting from low spacing values, increasing the distance between the dots increases the amplitude of the antisymmetric component field and thus of the coupling constant $\alpha_{\mathrm{as}}$, because for a fixed magnet thickness, a similar gradient can be extending over a longer length, until we reach a limit value. This limit comes from the geometry: the field difference is limited by the maximum values of the field that can be reached, of order $\mu_0 M_{\mathrm{s}}$ at most, when the dots are not contained in the same layer than the magnetic patterns. In practice, the spacing between the dots also cannot be increased unlimitedly, as we want the dots to have some overlap, with a sufficient tunneling rate. For two dots confined in a nanowire, 400 nm remains a reasonable value for the spacing between the dots [1], which could further enhance the field difference.

In Supp. Fig. S3(b), the thickness of the magnetic layer is varied for a fixed interdot spacing of 400 nm. Increasing the thickness of the magnetic layer allows to improve $\alpha_{\mathrm{as}}$ until we reach a maximum value. Above a thickness of 500 nm, the value of $\alpha_{\mathrm{as}}$ and thus the amplitude of the antisymmetric component field starts to saturate with the thickness of the magnetic layer. In the examples presented along the main of the article, a thickness of 200 nm is preferred as it simplifies the nanofabrication process and the integration of the double quantum dot on chips.

## S4. MICROMAGNETIC SIMULATIONS AND STATES AT EQUILIBRIUM

In order to obtain a uniform magnetization along any axis despite internal demagnetizing fields, it is advisable to induce a favourable shape anisotropy, while keeping unchanged the regions of the magnet contributing the most to $\alpha_{\mathrm{as}}$. This allows in turn to reduce the minimal external field (here along $x$) required to saturate the magnet. Comparing between the optimized shapes of saturated nanomagnets, a shape anisotropy is easier to obtain with the geometry optimizing the field difference along the $B_{\mathrm{z}}$ component. We thus use this shape, keeping for MuMax$^3$ simulations a width (along $y$) of 1 µm and a length (along $x$) of 7 µm, which are the largest dimensions that could be simulated considering our hardware access. To avoid the effects of this finite length of the magnetic layer in our simulations, while real magnets could be much longer, periodic boundary conditions are chosen in the $x$ direction. The magnetic parameters considered for the simulations are listed in Table S1.

TABLE S1. Magnetic parameters used in micromagnetic simulations.

| Material | $\mathrm{M_S}$ ($10^3\,\mathrm{A\,m^{-1}}$) | A ($10^{-12}\,\mathrm{J\,m^{-1}}$) | Shape | References |
|---|---|---|---|---|
| NiFe | 800 | 13 | 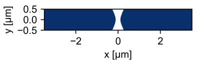  | [2], [3] |
| Co | 1450 | 56 | | [4], [3] |
| CoFe | 2000 | 20 | | [5], [3] |

To determine the micromagnetic configurations at equilibrium, we compute a configuration of minimal energy taking into account the exchange interaction between the spins, the internal dipolar interactions and the Zeeman energy. It is done for decreasing values of the external field, starting from magnetic saturation under a field of 1 T. We present in Supp. Fig. S4 two examples of minimal energy configurations that have been obtained. When saturation is lost, the reduction of the average $m_{\mathrm{x}}$ below 1 corresponds to the formation of closure domains at the extremities of the nanomagnets, affecting drastically the generated gradient.

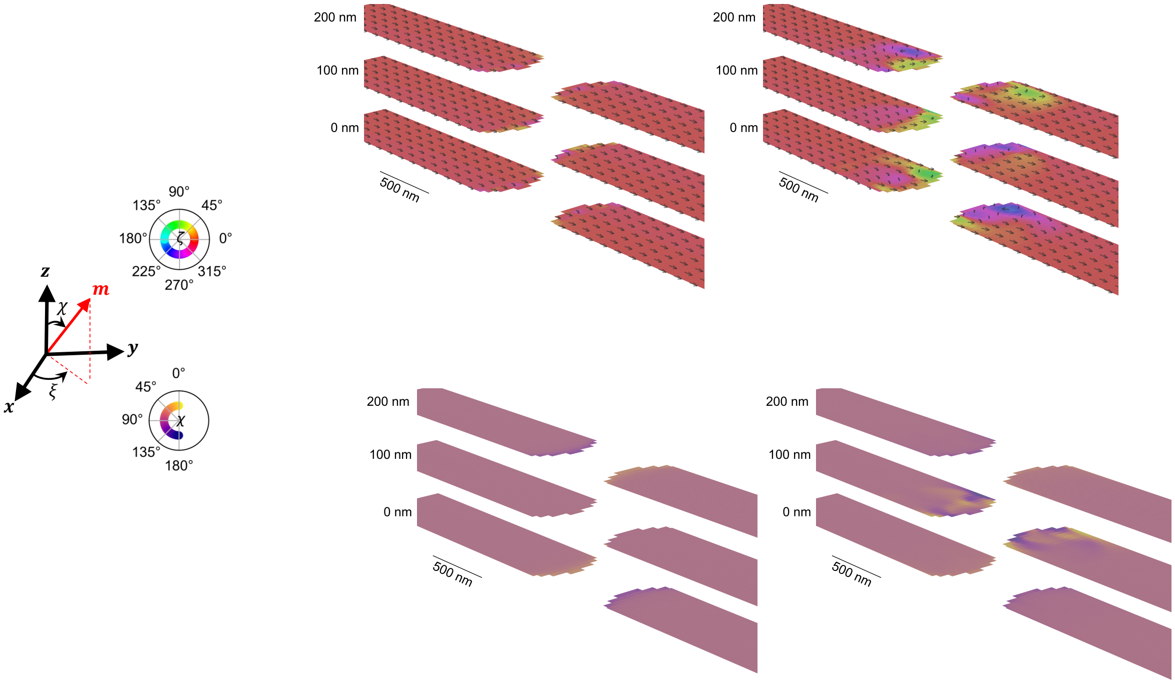


FIG. S4. Micromagnetic configurations obtained after energy minimization with Mumax[3], for the case of CoFe. We start by applying a large magnetic field of 1 T along the wires and then reduce the amplitude of the external field in steps of 0.1 T, to compute the configuration at equilibrium under a magnetic field of 0.5 T (left) and 0.1 T (right).

## S5. EXTRACTION OF THE STRAY FIELDS AND CALCULATION OF THE COUPLING CONSTANTS

From the above micromagnetic configurations, we are able to extract the stray fields at 100 nm above the surface of the magnetic layer, as was done for the saturated magnets case. From the linear profiles of the magnetic field $\mathbf{B}(x)$, examplified in Supp. Fig. S5, we can deduce the coupling constants $\alpha_{\rm s}$ and $\alpha_{\rm as}$.

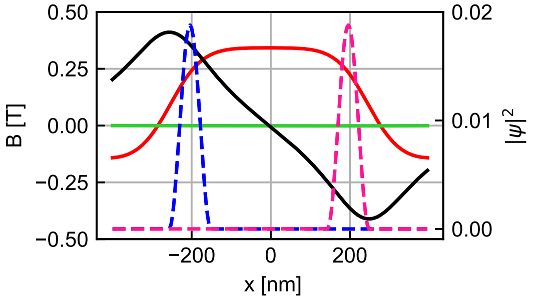


FIG. S5. Profile of the stray magnetic fields obtained from micromagnetic simulations in the case of CoFe nanomagnets, for (a) $B_{\rm ext} = 500\,\rm mT$ and (b) $B_{\rm ext} = 100\,\rm mT$. $B_x$ in red, $B_y$ in green and $B_z$ in black, and overlap with the probability of presence $|\psi_p(\mathbf{r})|^2$ of an electron in the left/right dot (respectively in blue/pink).


[1] T. Cubaynes, M. R. Delbecq, M. C. Dartiailh, R. Assouly, M. M. Desjardins, L. C. Contamin, L. E. Bruhat, Z. Leghtas, F. Mallet, A. Cottet, and T. Kontos, Highly coherent spin states in carbon nanotubes coupled to cavity photons, npj Quantum Inf. **5**, 47 (2019).

[2] N. Sorensen, R. Camley, and Z. Celinski, Exchange stiffness as a function of composition in $\mathrm{Cu}_x(\mathrm{Ni0.80Fe0.20})_{1-x}$ alloys, Journal of Magnetism and Magnetic Materials **477**, 344 (2019).

[3] T. Thomson, 10 - magnetic properties of metallic thin films, in *Metallic Films for Electronic, Optical and Magnetic Applications*, edited by K. Barmak and K. Coffey (Woodhead Publishing, 2014) pp. 454–546.

[4] M. D. Kuz'Min, K. P. Skokov, L. V. B. Diop, I. A. Radulov, and O. Gutfleisch, Exchange stiffness of ferromagnets, The European Physical Journal Plus **135**, 10.1140/epjp/s13360-020-00294-y (2020).

[5] H. S. Jung, W. D. Doyle, and S. Matsunuma, Influence of underlayers on the soft properties of high magnetization FeCo films, Journal of Applied Physics **93**, 6462 (2003), https://doi.org/10.1063/1.1557653.
